# Supplementary material for: Fast Convex Optimization for Two-Layer ReLU Networks: Equivalent Model Classes and Cone Decompositions
Source: arXiv:2202.01331 source file (2025-04-08)
Supplement: Supplementary file 1 [file active_set.tex]

%!TEX root = ../main.tex

\section{Active Set Strategies}\label{app:active-set}

In this section, we develop techniques for choosing or augmenting the set of sign patterns \( \tilde \calD \) for the C-ReLU or C-GReLU convex reformulations.
Recall from Section~\ref{sec:relu-models} that \( |\calD_X| \in O(r (n/r)^r )\) for \( r = \text{rank}(X) \);
it is computationally infeasible to take \( \tilde \calD = \calD_X \) when \( n \geq d \) and \( r \in O(d) \) since then \( |\calD_X| \) is exponential in the feature dimension.
However, it is still possible to leverage the theory of sub-sampled convex reformulations to obtain guarantees on the performance of the convex reformulations relative to a \emph{specific} non-convex model by choosing \( \tilde \calD \) carefully.
We find that doing so can also improve generalization in practice.

\subsection{Stochastic Optimization as an Active Set Method}

The simplest way to select \( \tilde \calD \) is to randomly sample generating vectors from a distribution on \( \R^d \).
For example, taking \( z_1, \ldots, z_m \stackrel{\text{\rm \tiny iid}}{\sim} \calN(0, \bfI) \), we obtain a valid set of sign patterns as
\[
	\tilde \calD = \cbr{\text{diag}(X z_i > 0) : i \in [m]},
\]
with the simple guarantee \( |\tilde \calD| \leq m \).
Note that it is useful to drop the zero matrix \( 0 * \bfI \), which introduces a \( d \)-dimensional subspace of equivalent models, and to filter out duplicate patterns.
In some applications, such as image classification, it is useful to generate sparse generating vectors that leverage spatial properties of the data (see Appendix~\ref{app:image-datasets-exp}).
However, these strategies yield no guarantees with respect to a non-convex model.

An alternative approach comes from viewing (stochastic) optimization of a ReLU network as an active set method in the space of activation patterns.
Let \( h_{W_1, w_2} \) be a two-layer neural network with ReLU activations with \( m < |\calD_X| \) neurons and consider optimizing the network with an arbitrary method that generates iterates \( \rbr{W_1^t, w_2^t} \).
The forward operator for the network at iteration \( t \) may be re-written as
\begin{align*}
	h_{W^t_1, w^t_2}(X)
	 & = \sum_{i \in [m]} \rbr{X W^t_{1i}}_+ w^t_{2i}                               \\
	 & = \sum_{i \in [m]} \text{diag}\rbr{X W^t_{1i} > 0} \rbr{X W^t_{1i}} w^t_{2i} \\
	 & = \sum_{i \in [m]} D_i^t \rbr{X W^t_{1i}} w^t_{2i},
\end{align*}
where \( \calA^t = \cbr{D^t_i = \text{diag}\rbr{X W^t_{1i} > 0} : i \in [m]} \) is the collection of ``active'' patterns.
We can also define \( \calI^t = \calD_X \setminus \calA^t \) to be the set of inactive patterns and an extended weight space
\begin{align*}
	\rbr{\bar W_{1i}^t, \bar w_{2i}^t} =
	\begin{cases}
		\rbr{W_{1i}^t, w_{2i}^t} & \mbox{if \( D_i \in \calA^t \)} \\
		\rbr{0, 0}               & \mbox{otherwise},
	\end{cases}
\end{align*}
which leads to the following version of the forward operator:
\begin{align*}
	h_{W^t_1, w^t_2}(X)
	 & = \sum_{D_i \in \calA^t} D_i \rbr{X \bar W^t_{1i}} \bar w^t_{2i} + \sum_{D_i \in \calI^t} D_i \rbr{X \bar W^t_{1i}} \bar w^t_{2i},
\end{align*}
Thus, the forward operator for non-convex ReLU network is equivalent to that of the convex reformulation with an additional constraint limiting the number of active sign-patterns to be at most \( m \) at every iteration.
In this interpretation, the learning procedure optimizes over both the active set and the weights \( \rbr{W_{1}, w_{2}} \).

The path of active sign patterns \( \rbr{\calA^t}_{t=0}^T \) provides an alternative way to generate \( \tilde \calD \).
In particular, we propose several simple strategies:
\begin{itemize}
	\item \textbf{Full Path}: choose \( \tilde \calD = \calD_0 \cup \rbr{\bigcup_{t=1}^T \calA^t} \), where \( \calD_0 \) is an initial ``diversity'' set generated by random sampling.
	\item \textbf{Final Activations}: choose  \( \tilde \calD = \calD_0 \cup \calA^T \).
	      This corresponds to taking only the activation patterns from the final non-convex model, i.e., the output of the non-convex optimization procedure.
	\item \textbf{Mixture of Experts}: choose  \( \tilde \calD = \calD_0 \cup \rbr{\bigcup_{s \in \calS} \calA_s^T} \), where \( \calS \) is a set of random seeds, optimization procedures, or architectures producing a diverse set of final models.
	      We interpret \( \bigcup_{s \in \calS} \calA_s^T \) as a sort of mixture-of-experts allowing \( \tilde \calD \) to incorporate information from different local minima or even different models.
\end{itemize}
These approaches treat non-convex optimization of the ReLU network as an algorithm for sampling from \( \calD_X \).
Note that restricting to two-layer networks (or neural networks at all) is unnecessary;
any method which partitions the rows of \( X \) into active and inactive sets achievable by a ReLU neuron is valid.

\subsection{Experimental Results}

\begin{table*}[t]
	\centering
	\begin{tabular}{lllllll} \toprule
		                 & \multicolumn{3}{c}{Training Objective} & \multicolumn{3}{c}{Test Accuracy}                                                                            \\ \cmidrule(r){2-4} \cmidrule(l){5-7}
		\textbf{Dataset} & \textbf{C-GReLU}                       & \textbf{C-ReLU}                   & \textbf{NC-ReLU} & \textbf{C-GReLU} & \textbf{C-ReLU} & \textbf{NC-ReLU} \\ \midrule
		statlog-heart    & 0.007 (0.01)                           & 0.019 (0.055)                     & 0.02             & 77.3 (77.3)      & 75.0 (74.4)     & 72.7             \\
		vertebral-col.   & 0.026 (0.076)                          & 0.156 (0.194)                     & 0.179            & 79.6 (81.6)      & 81.6 (84.0)     & 82.0             \\
		cardiotocogr.    & 0.033 (0.035)                          & 0.043 (0.046)                     & 0.074            & 91.5 (90.9)      & 88.5 (87.1)     & 91.2             \\
		abalone          & 0.094 (0.096)                          & 0.098 (0.1)                       & 0.248            & 63.5 (63.3)      & 61.7 (61.0)     & 65.3             \\
		car              & 0.04  (0.04)                           & 0.045 (0.046)                     & 0.116            & 81.2 (80.1)      & 76.5 (76.9)     & 88.1             \\
		breast-cancer    & 0.024 (0.034)                          & 0.066 (0.145)                     & 0.075            & 71.7 (65.2)      & 65.2 (67.4)     & 65.2             \\
		contrac          & 0.08  (0.092)                          & 0.095 (0.102)                     & 0.251            & 54.5 (55.1)      & 57.2 (53.6)     & 56.8             \\
		congressional    & 0.383 (0.384)                          & 0.385 (0.389)                     & 0.385            & 60.0 (58.6)      & 58.6 (60.0)     & 58.6             \\
		synthetic        & 0.01  (0.013)                          & 0.015 (0.019)                     & 0.037            & 99.0 (97.9)      & 99.0 (97.9)     & 97.9             \\
		musk-1           & 0.003 (0.005)                          & 0.007 (0.013)                     & 0.008            & 90.8 (85.5)      & 92.1 (88.3)     & 92.1             \\
		ecoli            & 0.015 (0.019)                          & 0.019 (0.021)                     & 0.086            & 90.6 (90.6)      & 88.9 (85.2)     & 90.7             \\
		hill-valley      & 0.197 (0.405)                          & 0.411 (0.412)                     & 0.458            & 57.7 (61.9)      & 63.9 (66.0)     & 57.7             \\ \bottomrule
	\end{tabular}
	\caption{Comparison of the full path active set strategy for C-ReLU and NC-ReLU against the same problems with a fixed set of 100 activation patterns (shown in parenthesis) and NC-ReLU solved with SGD.
		We report the median training objective and test accuracy from five-fold cross validation.
	}%
	\label{table:active-set-short}
\end{table*}

Now we provide preliminary results for the full path active set approach introduced in the previous section.
We test our ideas on a subset of twelve datasets from the UCI repository and provide results for NC-ReLU trained with SGD, C-GReLU with R-FISTA, and C-ReLU with our AL method.

For all methods, we use a fixed regularization parameter of \( \lambda = 10^{-4} \).
For the NC-ReLU problem, we use \( m = 100 \) and try initial step-sizes in the grid \( \cbr{10, 5, 1, 0.5, 0.1, 0.01} \).
Results are reported \emph{only} for the step-size which produced the smallest median training objective as determined by five-fold cross validation after \( 2000 \) epochs.
We also use a decay schedule that divides the step-size by two every \( 100 \) epochs to ensure that SGD has a chance of converging.
The mini-batch size is always \( 10\% \) of the dataset.

For the convex formulations, we use a diversity set \( \calD_0 \) of 100 sign patterns generated by randomly sampling Gaussian vectors as described above.
R-FISTA and our AL method are run with standard parameters (see Appendix~\ref{app:default-parameters}).
We report results for \( \tilde \calD = \calD_0 \) and the full path strategy to illustrate the effects of the active set approach.
For full path, we use the patterns generated by the best run of SGD as chosen using the procedure above \emph{on a fold-by-fold} basis.
This ensures the results are comparable.

\cref{table:active-set-short} shows a summary of the results.
Convex reformulations using only the fixed diversity set \( \calD_0 \) are shown in parentheses next to results for the active set approach.
We find that including the activation patterns from the full optimization path always leads to a model with smaller training objective than the non-convex model;
in contrast, NC-ReLU sometimes obtains a smaller training objective than C-ReLU when only \( 100 \) fixed patterns are used (e.g. \texttt{breast-cancer}).
This empirically confirms part of \cref{thm:duality-free}, but we must emphasize that such observations are \emph{only} valid for the binary datasets \texttt{statlog-heart}, \texttt{congressional-voting}, \texttt{breast-cancer}, \texttt{musk-1}, and \texttt{hill-valley} where we do not use the one-vs-all strategy to extend the convex reformulations to the multi-class setting.

Including the path of sign patterns can also improve test accuracy, notably on \texttt{musk-1}.
We conjecture that convex reformulations using the active-set strategy will improve over those with fixed \( \calD_0 \) on every dataset when the regularization strength is tuned individually for each problem and method.
Such tuning is necessary because increasing the size of \( \tilde \calD \) also increases model capacity.
We did not attempt this here because changing the regularization parameters necessarily makes the training objectives incomparable.
See Tables~\ref{table:active-set-gated-obj} to~\ref{table:active-set-relu-acc} for the same results with spread/variance information.

\begin{table*}
	\centering
	\begin{tabular}{llll} \toprule
		\textbf{Dataset} & \textbf{C-GReLU (Fixed)} & \textbf{C-GReLU (AS) } & \textbf{NC-ReLU}    \\ \midrule
		statlog-heart    & 0.01 (0.01/0.01)         & 0.007 (0.007/0.007)    & 0.02 (0.021/0.02)   \\
		vertebral-col.   & 0.076 (0.076/0.072)      & 0.026 (0.026/0.026)    & 0.179 (0.181/0.178) \\
		cardiotocogr.    & 0.035 (0.035/0.034)      & 0.033 (0.034/0.033)    & 0.074 (0.074/0.074) \\
		abalone          & 0.096 (0.096/0.095)      & 0.094 (0.095/0.094)    & 0.248 (0.249/0.246) \\
		car              & 0.04 (0.04/0.04)         & 0.04 (0.04/0.039)      & 0.116 (0.117/0.115) \\
		breast-cancer    & 0.034 (0.035/0.033)      & 0.024 (0.025/0.022)    & 0.075 (0.077/0.071) \\
		contrac          & 0.092 (0.092/0.09)       & 0.08 (0.081/0.08)      & 0.251 (0.252/0.248) \\
		congressional    & 0.384 (0.386/0.377)      & 0.383 (0.385/0.376)    & 0.385 (0.388/0.378) \\
		synthetic        & 0.013 (0.013/0.013)      & 0.01 (0.01/0.01)       & 0.037 (0.038/0.037) \\
		musk-1           & 0.005 (0.005/0.005)      & 0.003 (0.003/0.003)    & 0.008 (0.009/0.008) \\
		ecoli            & 0.019 (0.019/0.017)      & 0.015 (0.015/0.014)    & 0.086 (0.087/0.079) \\
		hill-valley      & 0.405 (0.406/0.399)      & 0.197 (0.204/0.193)    & 0.458 (0.458/0.456) \\ \bottomrule
	\end{tabular}
	\caption{Median \textbf{training objective} shown with upper and lower quartiles for C-GReLU with ("AS") and without ("Fixed") the full path active set strategy.}%
	\label{table:active-set-gated-obj}
\end{table*}

\begin{table*}
	\centering
	\begin{tabular}{llll} \toprule
		\textbf{Dataset} & \textbf{C-GReLU (Fixed)} & \textbf{C-GReLU (AS)} & \textbf{NC-ReLU} \\ \midrule
		statlog-heart    & 77.3 (81.4/74.4)         & 77.3 (79.1/72.1)      & 72.7 (79.1/72.1) \\
		vertebral-col.   & 81.6 (82.0/77.6)         & 79.6 (84.0/76.0)      & 82.0 (84.0/81.6) \\
		cardiotocogr.    & 90.9 (90.9/89.4)         & 91.5 (91.8/90.0)      & 91.2 (92.6/90.3) \\
		abalone          & 63.3 (63.5/62.0)         & 63.5 (64.8/63.1)      & 65.3 (66.3/64.9) \\
		car              & 80.1 (81.6/79.8)         & 81.2 (82.3/81.2)      & 88.1 (88.8/85.9) \\
		breast-cancer    & 65.2 (67.4/65.2)         & 71.7 (71.7/69.6)      & 65.2 (69.6/63.0) \\
		contrac          & 55.1 (57.2/55.1)         & 54.5 (55.1/50.8)      & 56.8 (57.4/56.8) \\
		congressional    & 58.6 (62.3/56.5)         & 60.0 (60.0/56.5)      & 58.6 (61.4/56.5) \\
		synthetic        & 97.9 (97.9/94.8)         & 99.0 (99.0/96.9)      & 97.9 (99.0/96.9) \\
		musk-1           & 85.5 (88.2/84.2)         & 90.8 (92.1/88.3)      & 92.1 (93.4/90.8) \\
		ecoli            & 90.6 (90.7/88.9)         & 90.6 (92.6/88.9)      & 90.7 (92.6/88.7) \\
		hill-valley      & 61.9 (64.9/60.8)         & 57.7 (62.9/57.7)      & 57.7 (60.8/55.7) \\ \bottomrule
	\end{tabular}
	\caption{Median \textbf{test accuracy} shown with upper and lower quartiles for C-GReLU with ("AS") and without ("Fixed") the full path active set strategy.}%
	\label{table:active-set-gated-acc}
\end{table*}

\begin{table*}
	\centering
	\begin{tabular}{llll} \toprule
		\textbf{Dataset} & \textbf{C-ReLU (Fixed)} & \textbf{C-ReLU (AS) } & \textbf{NC-ReLU}    \\ \midrule
		statlog-heart    & 0.055 (0.056/0.05)      & 0.019 (0.02/0.019)    & 0.02 (0.021/0.02)   \\
		vertebral-col.   & 0.194 (0.198/0.193)     & 0.156 (0.159/0.154)   & 0.179 (0.181/0.178) \\
		cardiotocogr.    & 0.046 (0.047/0.046)     & 0.043 (0.043/0.042)   & 0.074 (0.074/0.074) \\
		abalone          & 0.1 (0.101/0.1)         & 0.098 (0.099/0.098)   & 0.248 (0.249/0.246) \\
		car              & 0.046 (0.046/0.046)     & 0.045 (0.045/0.044)   & 0.116 (0.117/0.115) \\
		breast-cancer    & 0.145 (0.145/0.14)      & 0.066 (0.067/0.064)   & 0.075 (0.077/0.071) \\
		contrac          & 0.102 (0.103/0.101)     & 0.095 (0.095/0.094)   & 0.251 (0.252/0.248) \\
		congressional    & 0.389 (0.391/0.381)     & 0.385 (0.387/0.378)   & 0.385 (0.388/0.378) \\
		synthetic        & 0.019 (0.019/0.019)     & 0.015 (0.015/0.015)   & 0.037 (0.038/0.037) \\
		musk-1           & 0.013 (0.013/0.013)     & 0.007 (0.007/0.007)   & 0.008 (0.009/0.008) \\
		ecoli            & 0.021 (0.021/0.021)     & 0.019 (0.019/0.018)   & 0.086 (0.087/0.079) \\
		hill-valley      & 0.412 (0.414/0.409)     & 0.411 (0.416/0.41)    & 0.458 (0.458/0.456) \\ \bottomrule
	\end{tabular}
	\caption{Median \textbf{training objective} shown with upper and lower quartiles for C-ReLU with ("AS") and without ("Fixed") the full path active set strategy.}%
	\label{table:active-set-relu-obj}
\end{table*}

\begin{table*}
	\centering
	\begin{tabular}{llll} \toprule
		\textbf{Dataset} & \textbf{C-ReLU (Fixed)} & \textbf{C-ReLU (AS)} & \textbf{NC-ReLU} \\ \midrule
		statlog-heart    & 74.4 (81.4/72.1)        & 75.0 (81.4/69.8)     & 72.7 (79.1/72.1) \\
		vertebral-col.   & 84.0 (86.0/83.7)        & 81.6 (86.0/80.0)     & 82.0 (84.0/81.6) \\
		cardiotocogr.    & 87.1 (87.6/87.1)        & 88.5 (89.1/88.2)     & 91.2 (92.6/90.3) \\
		abalone          & 61.0 (62.3/60.8)        & 61.7 (63.6/61.2)     & 65.3 (66.3/64.9) \\
		car              & 76.9 (78.7/74.7)        & 76.5 (78.7/75.8)     & 88.1 (88.8/85.9) \\
		breast-cancer    & 67.4 (69.6/63.0)        & 65.2 (69.6/65.2)     & 65.2 (69.6/63.0) \\
		contrac          & 53.6 (55.1/53.0)        & 57.2 (57.4/55.5)     & 56.8 (57.4/56.8) \\
		congressional    & 60.0 (62.9/56.5)        & 58.6 (58.6/58.0)     & 58.6 (61.4/56.5) \\
		synthetic        & 97.9 (99.0/96.9)        & 99.0 (99.0/95.8)     & 97.9 (99.0/96.9) \\
		musk-1           & 88.3 (89.5/86.8)        & 92.1 (94.7/89.5)     & 92.1 (93.4/90.8) \\
		ecoli            & 85.2 (90.7/85.2)        & 88.9 (88.9/86.8)     & 90.7 (92.6/88.7) \\
		hill-valley      & 66.0 (67.0/63.9)        & 63.9 (64.9/61.9)     & 57.7 (60.8/55.7) \\ \bottomrule
	\end{tabular}
	\caption{Median \textbf{test accuracy} shown with upper and lower quartiles for C-ReLU with ("AS") and without ("Fixed") the full path active set strategy.}%
	\label{table:active-set-relu-acc}
\end{table*}
